# Supplementary material for: Mind the Gap Between Conversations for Improved Long-Term Dialogue Generation
Source: arXiv:2310.15415 source file (2023-10-24)
Supplement: Supplementary file 3 [file appendix_F.tex]

\section{Human Evaluation Questionnaire}
\label{apx_f}

We ask the annotators in total 11 questions and ask them to choose
\begin{table*}[]
    \centering
    \begin{tabular}{l}
    \toprule
    \textbf{Questions} \\
    \midrule
    \textit{Naturalness} \\
    \midrule
    Which dialogue do you think is more natural?   \\
    Which dialogue do you think is more like a dialogue between normal friends? \\
    In which dialogue do you think the speaker B talks more naturally? \\
    \midrule
    \textit{Informativeness} \\
    \midrule
    Which dialogue do you think provide more information about the speakers' daily events?    \\
    Which dialogue do you think is more efficient in updating the current status of the speakers?\\
    In which dialogue do you think the speaker B cares more about speaker A's daily events?\\
    \midrule
    \textit{Relevance} \\
    \midrule
    Does the speaker asks/talks about relevant events? \\
    Which dialogue do you think sticks to the topics of updating events? \\
    Do you think the speaker chooses natural, relevant events to talk about? \\
    \midrule
    \textit{Time-awareness} \\
    \midrule
    In which dialogue do you think you can identify a time gap? \\
    In which dialogue do you think the speaker B asks annoying questions more frequently? \\
    \bottomrule
    \end{tabular}
    \caption{The questions we ask annotators for the human evaluation.}
    \label{tab:questionnaire}
\end{table*}
